# Supplementary material for: Not Just Reason, Not Just Scan: Reinforcement Learning for Proactive Scientific Error Verification over Academic Paper
Source: arXiv:2608.26596 source file (2026-08-27)
Supplement: Supplementary file 1 [file d.tex]

\section{Use of LLMs}
\label{app:appendix_d}
We used LLM services for the experiments and data-processing procedures described in the paper. Gemini 3.0 Pro and GPT-5.4 were accessed through OpenRouter. Qwen3-VL-8B-Instruct and our trained Qwen3-VL-8B variants were evaluated locally on 4$\times$A800 GPUs. Seed-family models, including Seed-1.6-Thinking, were accessed through Volcano Engine. The remaining closed-source models and larger Qwen3-VL variants were accessed through Alibaba Cloud Bailian.
